# Supplementary material for: Deep Anomaly Detection in Text
Source: arXiv:2401.02971 source file (2023-12-14)
Supplement: Supplementary file 1 [file appendix1.tex]

\chapter{Cod sursă}

% XXX: BlazeDS config files
\section{Fișierele de configurare
	\label{anx.cfg}}
\subsection{Configurarea serviciilor}
\noindent
\ttfamily
\hlstd{}\hlkwa{$<$?xml\ }\hlstd{}\hlkwb{version}\hlstd{=}\hlstr{"1.0"}\hlstd{\ }\hlkwb{encoding}\hlstd{=}\hlstr{"UTF{-}8"}\hlstd{}\hlkwa{?$>$}\hspace*{\fill}\\
\hlstd{}\hlkwa{$<$services{-}config$>$}\hspace*{\fill}\\
\hlstd{}\hlstd{\ \ }\hlstd{}\hlkwa{$<$services$>$}\hspace*{\fill}\\
\hlstd{}\hlstd{\ \ \ \ }\hlstd{}\hlkwa{$<$service{-}include\ }\hlstd{}\hlkwb{file{-}path}\hlstd{=}\hlstr{"remoting{-}config.xml"}\hlstd{\ }\hlkwa{/$>$}\hspace*{\fill}\\
\hlstd{}\hlstd{\ \ \ \ }\hlstd{}\hlkwa{$<$default{-}channels$>$}\hspace*{\fill}\\
\hlstd{}\hlstd{\ \ \ \ \ \ }\hlstd{}\hlkwa{$<$channel\ }\hlstd{}\hlkwb{ref}\hlstd{=}\hlstr{"my{-}amf"}\hlstd{}\hlkwa{/$>$}\hspace*{\fill}\\
\hlstd{}\hlstd{\ \ \ \ }\hlstd{}\hlkwa{$<$/default{-}channels$>$}\hspace*{\fill}\\
\hlstd{}\hlstd{\ \ }\hlstd{}\hlkwa{$<$/services$>$}\hspace*{\fill}\\
\hlstd{}\hlkwa{$<$/services{-}config$>$}\hlstd{}\hspace*{\fill}\\
\mbox{}
\normalfont
